# Supplementary material for: Fair-CDA: Continuous and Directional Augmentation for Group Fairness
Source: arXiv:2304.00295 source file (2023-04-01)
Supplement: Supplementary file 1 [file appendix.tex]

\section{Datasets and Implementation Details}\label{sec:implementation}

\noindent\textbf{Adult.} Adult dataset contains information about over 40,000 individuals from the 1994 US Census. The classification task is to predict whether the income of a person is greater than 50K USD per year. The attribute information contains age, gender, education, occupation, etc. We consider gender as the sensitive attribute to evaluate fairness. 
Following~\citet{chuang2021fair}, we use a two-layer MLP with hidden size 200 as the backbone network and select the features from the hidden layer to apply decomposition. Similar to~\citet{chuang2021fair}, we retrain each model 10 times and report the mean accuracy and fairness metrics on the testing set.
In each trial, the training, validation and test sets account for 60\%, 20\% and 20\% of the total dataset respectively. 
The iterations of the training phase are 450, and that of fine-tuning phase is 10. Both models are optimized with Adam optimizer, the learning rate of the training process is $1\mathrm{e}{-3}$. and that of fine-tuning is $5\mathrm{e}{-4}$. For both DP and EO, we sample 500 data points from each protected group to form a batch.

\noindent\textbf{CelebA.} CelebA dataset contains over 200,000 images of celebrity
faces, where each image is associated with 40 human-labelled binary attributes. We also consider gender as a sensitive attribute to evaluate fairness. Following~\cite{chuang2021fair}, we select smiling, wavy hair and attractive to perform three binary classification tasks. For each task, we train a ResNet-18~\cite{he2016deep} as the backbone network. We select the features from  the last convolution layer to apply decomposition. We train the imputation model for 10 epochs and fine-tune the task model for 5 epochs. We use the original validation set of CelebA to perform model selection and report the accuracy and fairness metrics on the testing set. The optimizer is Adam, the learning rate of the training process is $1\mathrm{e}{-3}$ and that of fine-tuning is $4\mathrm{e}{-5}$. For both DP and EO, we sample 64 data points from each protected group to form a batch. For CelebA Heavy-Makeup recognition task, we implement Fair-CDA following the setting in~\cite{creager2019flexibly}.

\noindent\textbf{MovieLens.} MovieLens is a typical dataset used in recommender systems. It contains 1,000,209 anonymous ratings of approximately 3,900 movies made by 6,040 users. The users are annotated with demographic variables, and the movies are annotated with a set of attributes including producers, which are the providers of the content. We consider the producer as the sensitive attribute to evaluate fairness. 
To measure producer fairness, we divide the producers into the majority and minority groups according to the frequency of appearance. The producers appear more than 100 times in this dataset are regarded as the majority producer, and the remaining producers are regarded as the minority producer. 
Similar to the previous two datasets, we consider a binary classification task to recognize the rating of the movie, 5-star and 4-star ratings are regarded as positive feedbacks and labelled with 1, and the rest are labelled with 0. We use Deep and Cross Network (DCN)~\cite{wang2017deep} as the backbone network and choose the combination of the output features from cross-network and deep network to apply decomposition. We train the imputation model for 20 epochs and fine-tune the task model for 10 epochs. The dataset is randomly split into training, validation and testing sets with partitions 65\%,15\% and 20\%. We use the validation set to perform model selection and report the accuracy and fairness metrics on the testing set. The optimizer is Adam, the learning rate of the training process is $1\mathrm{e}{-3}$ and that of fine-tuning is $5\mathrm{e}{-4}$. For both DP and EO, we sample 256 data points from each protected group to form a batch.

\subsection{Range of Perturbation Strength} 
Fair-CDA mitigates the disparities of model predictions between different groups and balances the prediction accuracy and fairness via adjusting the perturbation strength $\lambda$. Intuitively, when we use a small value of $\lambda$, the augmented sensitive features will be close to the original features and the task model will have higher prediction accuracy. In contrast, when we use a large value of $\lambda$, the sensitive features will be changed to the features corresponding to the opposite sensitive attribute and the task model will have better fairness. 
The ranges of perturbation strength $\lambda$ are used to generate the Pareto Fronts on different datasets in our experiments, together with the recommended value of $\lambda$ that balances the accuracy and fairness well, are listed in Table~\ref{table:hyperparameter}. We also provide the ranges of weights that balance the classification loss and the regularization term for Fair Mixup~\cite{chuang2021fair}, GapReg~\cite{chuang2021fair} and AdvDebias~\cite{zhang2018mitigating} on MovieLens in Table~\ref{table:hyperparameter}.

\begin{table}[h]
\centering
\caption{Ranges and recommended value of trade-off parameters that balance the accuracy and fairness for different methods on Adult, CelebA and MovieLens.}
\label{table:hyperparameter}
    \begin{adjustbox}{max width=0.47\textwidth}
        \begin{tabular}{lllcc}
            \hline
            \hline
            Dataset & Method & Trade-off Parameter  & Range & Recommended Value \\
           \hline
            Adult	& Fair-CDA & Perturbation Strength  & [0,1000] & 500\\
            \hline
            CelebA	& Fair-CDA & Perturbation Strength   & [0,1000] & 500\\
            \hline
            \multirow{4}{*}{MovieLens} & Fair-CDA   & Perturbation Strength   & [0,10] & 1    \\	
                                       & Fair Mixup & Weight Balancing Losses & [0,10] & 0.2  \\
                                       & GapReg     & Weight Balancing Losses & [0,10] & 0.2  \\
                                       & AdvDebias  & Weight Balancing Losses & [0,10] & 0.2  \\
            \hline\hline
        \end{tabular}
    \end{adjustbox}
    %\vspace{-5pt}
\end{table}

\subsection{Network Architecture of Fair-CDA}

\noindent\textbf{Network architecture.} Fair-CDA is a general method that can be applied to various neural network models. On Adult, we use a \textbf{two-layer MLP} with hidden size 200 as the backbone network. The extracted features are then decomposed into non-sensitive and sensitive features using two fully-connected layers of size 200 respectively. Each fully-connected layer is followed by a fully-connected classification layer to predict the class label or sensitive attribute. The non-sensitive features and the augmented sensitive features are then concatenated together, followed by a fully-connected classification layer to make the final prediction. On the CelebA, we adopt \textbf{ResNet-18}~\cite{he2016deep} (without the final classification layer) as the backbone network. The output features are of dimension 512. The following two-branch architecture is the same as that used on Adult, except that the dimension of non-sensitive and sensitive features is 512. On MovieLens, we use \textbf{Deep and Cross Network (DCN)}~\cite{wang2017deep} as the backbone network. DCN has two networks: cross-network and deep network. We perform feature decomposition on the concatenation of the outputs from two networks. The concatenated features are of dimension 164. The following architecture for decomposition is the same as that we use on Adult, except that the dimension of non-sensitive and sensitive features is 164. The network architectures of Fair-CDA for different tasks are summarized in Table~\ref{table:decomposition}.

\begin{table}[t]
\centering
\caption{Network architectures of Fair-CDA used for different tasks. $Dim$ (Non-sensitive) and $Dim$ (Sensitive) denote the dimension of non-sensitive and sensitive features, respectively.}
\label{table:decomposition}
    \begin{adjustbox}{max width=0.47\textwidth}
        \begin{tabular}{lccc}
        \hline
        \hline
        Dataset & Backbone Network & $Dim$ (Non-sensitive) &  $Dim$ (Sensitive) \\
        \hline
        Adult	& Two-layer MLP & 200 & 200	 \\
        \hline
        CelebA	& ResNet-18 & 512 & 512  \\
        \hline
        MovieLens	& DCN   &  164 & 164 \\
        \hline
        \hline
        \end{tabular}
    \end{adjustbox}
    \vspace{-5pt}
\end{table}

\begin{table}
    \centering
    \caption{Parameter quantity comparison.}
    \label{table:para_ablation}
    % \vspace{-0.15cm}
	%\begin{adjustbox}{max width=0.9\textwidth}
        \begin{tabular}{lcc}
        \hline
        \hline
        Dataset &  Backbone Network &  Parameter Quantity  \\
        \hline
        Adult  & Two-layer MLP &  64,601  \\
               & Fair-CDA      &  146,005   \\
        \hline
        CelebA & ResNet-18     & 11,439,681 \\
               & Fair-CDA      & 11,967,557 \\
        \hline
        MovieLens & DCN        & 107,462 \\
                  & Fair-CDA   & 162,406 \\
        \hline
        \hline
        \end{tabular}
    %\end{adjustbox}
    %\vspace{-5pt}
\end{table}

\noindent\textbf{Additional parameters.} Since the task model is fine-tuned based on the trained imputation model, the additional parameters of the proposed method come from the two feature decomposition branches, i.e., two fully-connected layers and two classification layers, and one additional last classification layer to predict the labels for the augmented samples. The number of additional parameters is determined by the output dimension of the backbone and the dimensions of the sensitive / non-sensitive features. The statistics of parameter quantity are given in Table~\ref{table:para_ablation}.  

To do a fair comparison, we implement Fair Mixup with a two-layer wider MLP backbone (changing the hidden dimension from 200 to 400) on the Adult dataset. Similarly, we report the results under the same evaluation metrics and also compare the parameter quantity, as shown in Table~\ref{table:para_ablation_2}. we can see Fair-CDA still outperforms Fair Mixup. The performance gain mainly comes from the design of the method. Moreover, on the CelebA dataset, the parameter quantity of Fair-CDA is very close to that of the baseline model, we can still see significant improvement under both accuracy and fairness measurement.

\begin{table}[t]
    \centering
    \caption{Comparison between Fair-CDA and Fair Mixup with Wider MLP.}
    \label{table:para_ablation_2}
	\begin{adjustbox}{max width=0.47\textwidth}
        \begin{tabular}{lcccc}
        \hline
        \hline
        Method & $\Delta_{DP}$ & AP& $\Delta_{EO}$ &AP  \\
        \hline
        Fair Mixup with Wider MLP    & 0.024  &	0.728  & 0.046  & 0.763\\
        Parameter Quantity: 209,201  & 0.056  &	0.754  & 0.093  & 0.773\\
                                     & 0.141  &	0.781  & 0.134  & 0.777\\
        \hline
        Fair-CDA  & 0.022	& 0.783	  & 0.010   & 0.783 \\
        Parameter Quantity: 146,005   & 0.046   & 0.786   & 0.013   & 0.785\\
                  & 0.104	& 0.788	  & 0.032   & 0.787\\
        \hline
        \hline
        \end{tabular}
    \end{adjustbox}
    \vspace{-5pt}
\end{table}

\subsection{Training Procedure of Fair-CDA}

The training procedure of Fair-CDA consists of two stages, the training of the imputation model and the fine-tuning of the task model. 

\begin{table}
%    \vspace{-5pt}
    \centering
    \caption{Comparison between Fair-CDA and Fair-CDA without gradient orthogonalization loss.}
    \label{table:orth_loss}
	%\begin{adjustbox}{max width=0.9\textwidth}
        \begin{tabular}{lcccc}
        \hline
        \hline
        Method & $\Delta_{DP}$ & AP& $\Delta_{EO}$ &AP  \\
        \hline
        Fair-CDA                 & 0.038  &	0.770  & 0.041  & 0.776\\
        Without Gradient         & 0.087  &	0.778  & 0.057  & 0.782\\
        Orthogonalization Loss   & 0.097  &	0.782  & 0.175  & 0.785\\
        \hline
        Fair-CDA                 & 0.022   & 0.783	  & 0.010   & 0.783 \\
        With Gradient            & 0.046   & 0.786   & 0.013   & 0.785\\
        Orthogonalization Loss   & 0.104   & 0.788	  & 0.032   & 0.787\\
        \hline
        \hline
        \end{tabular}
    %\end{adjustbox}
%    \vspace{-5pt}
\end{table}

\noindent\textbf{Training of imputation model.} The training of the imputation model includes the following steps. First, we use the same network structure as the task model with feature decomposition in each experiment setting. Second, we train the imputation model with the original training data until convergence. Third, We save the imputation model and freeze the parameters.

\noindent\textbf{Fine-tuning of task model.} The fine-tuning of the task model includes the following steps. First, the task model is initialized based on the trained imputation model. Second,
the features extracted from original data are performed feature-level augmentation to augment features. Third, for the augmented features, the pseudo labels generated by the imputation model and the original labels are both used for fine-tuning the task model. 

\noindent\textbf{Fair-CDA without gradient orthogonalization loss.} The purpose of adding the gradient orthogonalization loss is to better decompose the features. We hope that the model can extract sensitive features that will not affect the label prediction loss and non-sensitive features that will not affect the sensitive attribute prediction loss. We also conduct experiments without the gradient orthogonalization loss on the Adult dataset and the results are illustrated in Table~\ref{table:orth_loss}. It can be seen that the regularization loss improves fairness a lot.

\section{More Related Work}

\noindent\textbf{Fair Machine Learning.} 
Fair machine learning methods can be classified into three types according to their different phases of application: pre-processing, in-processing, and post-processing. In particular, in-processing methods contain representation learning and fairness-aware models~\cite{ekstrand2021fairness}. 

\citet{Kamiran2012} propose four different methods for pre-processing: suppression, massaging, reweighing, and resampling. 
Suppression removes sensitive attributes and those most correlated to sensitive attributes to eliminate existing discrimination. Massaging changes the labels of certain samples to minimize the discrimination from the input data, similar to~\cite{2009Classifying}. Reweighing and resampling change the weight or distribution of certain inputs, instead of changing the labels. 

Fair representation learning aims to map the input distribution to a latent distribution that can encode the data as well as possible, and obfuscate or remove any information about sensitive attributes simultaneously. In~\cite{Zemellearningfair}, probabilistic mapping is used to guarantee the probability that a data point map from a specific group to a particular prototype is equal to that from another group. In ~\cite{lahoti2019ifair}, matrix transformation is applied to learn the fair representation.
Moreover, methods formulating non-discriminatory representation learning as a goal in adversarial training are proposed in~\cite{feng2019learning,madras2018learning}. 
To train a fairness-aware model, Gap Regularization~\cite{chuang2021fair} directly adds fairness objective penalty terms to the loss function to satisfy specific fairness constraints. 
Fair Mixup~\cite{chuang2021fair} adopts mixup of samples in input space or mixup of features in latent space. It regularizes the models on paths of interpolated samples between different groups to improve the generalization for both accuracy and fairness. 

Post-processing methods mainly deal with the output predictions,
operating in a black-box fashion. According to~\cite{zhou2021bias}, such algorithms require the protected attributes to be available in the usage stage, which will introduce compliance risks.

\noindent\textbf{Fair Representation Learning.}
Current solutions for imposing fairness constraints can be classified into causal based approaches \cite{khademi2019fairness,kusner2017counterfactual}, ranking based models \cite{beutel2019fairness}, and fair representation learning models \cite{bose2019compositional,edwards2015censoring,madras2018learning,Zemellearningfair}. 
Fair representation learning is a rapid progress technique of representation learning that protects task models from the potentially harmful effects that sensitive features may have on the classification task \cite{hardt2016equality,mcnamara2017provably,locatello2019fairness}.
\citet{Zemellearningfair} and \citet{dwork2011fairness} establish that a fair representation should preserve all information about the main task with the exception of direct or indirect information arising from sensitive attributes.
There are several approaches that employ adversarial training \cite{goodfellow2014generative}
to prevent sensitive information from being leaked into the representation \cite{edwards2015censoring,madras2018learning,zhang2018mitigating,xu2018fairgan,feng2019learning}.
In this work, we also use adversarial training to augment a path of distributions that connects sensitive groups. 
Similar to \citet{chuang2021fair}, our method ensures a better generalization for both accuracy and fairness in a wide range of benchmarks.
Here we focus on the adversarial methods. For more related works, please refer to \cite{louizos2015variational,calmon2017optimized,song2019learning,kusner2017counterfactual,joachims2016counterfactual} and so on.

\noindent\textbf{Feature Disentanglement.} 
Introducing invariance against sensitive attributes while performing well on specific tasks is an important problem in representation learning. This can be addressed by feature disentanglement and cleaning the sensitive information from learned representations \cite{sarhan2020fairness,park2021learning,jha2021fair,li2022towards,quadrianto2019discovering}. 
Similar to fair representation disentanglement, OOD methods aim to learn invariant representations across different domains and identify stable and invariant relationships between features and targets. IRM~\cite{arjovsky2019invariant} extracts invariant representations by adding an invariant risk regularization term to the loss function. MASF~\cite{dou2019domain} adopts a meta-learning procedure to extract invariant features across domains. DGBR~\cite{Kuang2018} jointly learns a global balancing model and a deep auto-encoder model for stable prediction across unknown environments. DecAug~\cite{bai2020decaug} explicitly decomposes the features into category-related and context-related parts by predicting category and context labels, respectively. An orthogonality constraint on the gradients of the two prediction losses is added to better decompose the features. We also adopt the gradient orthogonalization loss to do feature decomposition and reduce the dependence of model predictions on the sensitive attributes.
